# Supplementary material for: Neural network interpolation of exchange-correlation functional
Source: arXiv:1909.03860 source file (2019-10-14)
Supplement: Supplementary file 1 [file supplementary.pdf]

Electronic Supplementary Material (ESI) for Physical Chemistry Chemical Physics
This journal is © The Owner Societies 2019

Supplementary information

# Neural network interpolation of exchange-correlation functional

*Alexander Ryabov,*[1,2] *Petr Zhilyaev*[*2]

[1] Moscow Institute of Physics and Technology (State University), Institutskiy per. 9, Dolgoprudny, Moscow Region 141700, Russia

[2] Center for Design, Manufacturing and Materials, Skolkovo Institute of Science and Technology, Skolkovo Innovation Center, Building 3, Moscow, 143026, Russia; E-mail: p.zhilyaev@skoltech.ru

S1

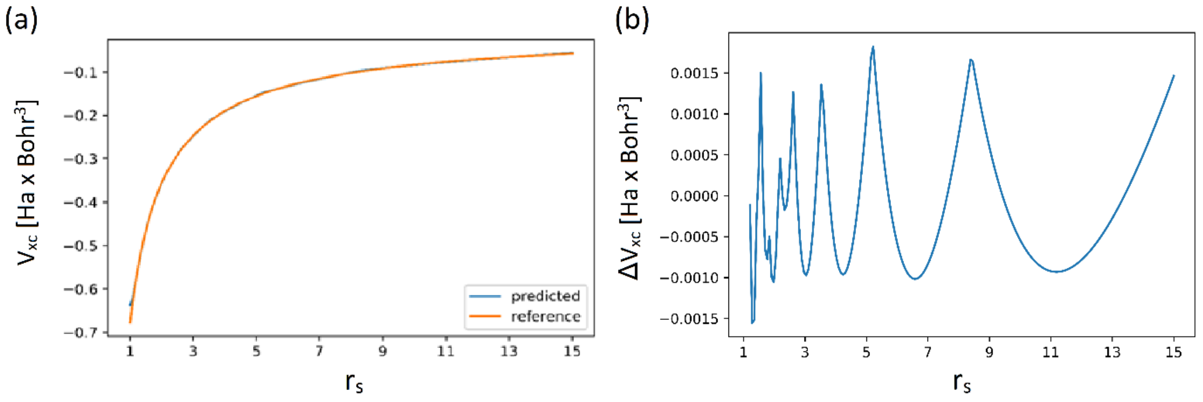


*Figure S1*. (a) LDA exchange-correlation potential versus $r_s$. Blue line – exchange-correlation potential obtained from NN, orange line – reference analytical LDA exchange-correlation potential. (b) Difference between exchange-correlation obtained from NN and reference analytical LDA exchange-correlation potential.

S2

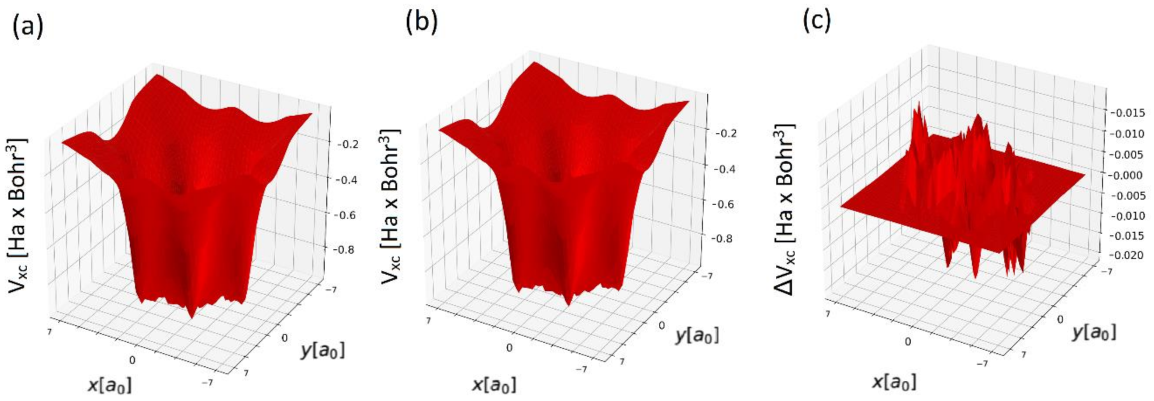


*Figure S2*. (a) Slice of LDA exchange-correlation initial potential obtained by NN for benzene at z = 0. (b) Slice of LDA exchange-correlation potential for benzene obtained by NN from 5x5x5 density cube which rotated by 90 degrees along z axis passing through the centre of the cube. (c) Difference between slices specified in (a) and (b)
